# Supplementary material for: High-throughput analysis of Fr\"ohlich-type polaron models
Source: arXiv:2207.00364 source file (2022-07-01)
Supplement: Supplementary file 1 [file supinfo.pdf]

# High-throughput analysis of Fröhlich-type polaron models

Pedro Miguel M. C. de Melo[1,2], Joao C. de Abreu[2], Bogdan Guster[3], Matteo Giantomassi[3], Zeila Zanolli[1], Xavier Gonze[3], and Matthieu J. Verstraete[2]

[1] *Chemistry Department, Debye Institute for Nanomaterials Science and European Theoretical Spectroscopy Facility, Condensed Matter and Interfaces, Utrecht University, PO Box 80.000, 3508 TA Utrecht, The Netherlands*

[2] *nanomat/Q-MAT/CESAM and European Theoretical Spectroscopy Facility, Université de Liège, B-4000 Liège, Belgium and*

[3] *UCLouvain, Institute of Condensed Matter and Nanosciences (IMCN), Chemin des Étoiles 8, B-1348 Louvain-la-Neuve, Belgium*

(Dated: June 30, 2022)

## S. METHODS AND CODES

From the high-throughput calculations within the Fröhlich model we focus on a few materials calculated within the non-adiabatic Allen, Heine, Cardona (AHC)[1,2] theory. Comparing the two approaches, the former only includes long-wavelength fields of longitudinal optical phonons, while excluding short-range fields, non-LO vibration modes, second-order coupling to the atomic displacements, also known as the Debye-Waller (DW) self-energy, inter-band contributions and non-parabolic effective masses which are included in the latter.

The electronic and phonon properties were calculated using ABINIT. To quantify the interaction between phonons and electrons we apply the lowest order of many-body perturbation theory which is sufficient[3] to describe the electron-phonon interactions in the quasi-particle self-energy. The self-energy contains two terms: the static Debye-Waller (DW),[4] and the dynamic Fan (FAN)[5] terms,

$$\Sigma_{\mathbf{k}n}(\omega) = \Sigma^{\mathrm{DW}}_{\mathbf{k}n} + \Sigma^{\mathrm{FAN}}_{\mathbf{k}n}(\omega). \tag{S.1}$$

The non-adiabatic AHC ZPR is obtained directly from the real part of the self-energy evaluated at the Kohn-Sham (KS) using Density Functional Theory (DFT) electronic energy $\varepsilon_{\mathbf{k}n}$ in a state defined by the wave-vector $\mathbf{k}$ and the band $n$,

$$\mathrm{ZPR}_{\mathbf{k}n} = \Re e \Sigma \left(\omega = \varepsilon_{\mathbf{k}n}\right). \tag{S.2}$$

The non-adiabatic method includes the contribution of the phonons frequencies to the Fan denominator, representing the retarded movement of the electrons forced by the ionic motion, and at 0 K temperature it can be described as

$$\begin{aligned}\Sigma^{\mathrm{Fan}}_{\mathbf{k}n}(\omega) = \frac{1}{N_q}\sum_{\mathbf{q}}^{\mathrm{BZ}}\sum_{j}\sum_{n'}\left|\left\langle \mathbf{k}+\mathbf{q}n'\left|H^{(1)}_{\mathbf{q}j}\right|\mathbf{k}n\right\rangle\right|^2 \times \\ \left[\frac{1-f_{\mathbf{k}+\mathbf{q}n'}}{\omega-\varepsilon_{\mathbf{k}+\mathbf{q}n'}-\omega_{\mathbf{q}j}+i\eta}+\frac{f_{\mathbf{k}+\mathbf{q}n'}}{\omega-\varepsilon_{\mathbf{k}+\mathbf{q}n'}+\omega_{\mathbf{q}j}+i\eta}\right].\end{aligned} \tag{S.3}$$

The phonon's contributions to the self-energy are included in the sum of the phonon frequencies, $\omega_{\mathbf{q}j}$, over the phonon wavevectors $\mathbf{q}$ in the Brillouin Zone and the phonon modes $j$. There is also the contribution of the scattering of electron from state $|\mathbf{k}n\rangle$ to the state $|\mathbf{k}+\mathbf{q}n'\rangle$ due to the perturbation $H^{(1)}$ of the $\mathbf{q}j$ phonon. These terms are determined within Density Functional Perturbation Theory (DFPT). The scattered potentials in $H^{(1)}$ is first calculated in a coarse q-mesh grid and then interpolated to a finer q-mesh. In this Fourier-based interpolation, we removed the dipole and quadrupole terms before the interpolation to treat the non-analytical behaviour at long wave-length and added them after, more details can be found in Refs. 6–8.

In Section IV, we will split $\Sigma^{\mathrm{Fan}}_{\mathbf{k}n}$ into its wave-vector $\mathbf{q}$ or phonon mode $j$ components and remove the sum in eq. S.3 of the correspondent component. The self-energy becomes $\Sigma^{\mathrm{Fan}}_{\mathbf{qk}n}$ or $\Sigma^{\mathrm{Fan}}_{j\mathbf{k}n}$, respectively. Separating the FAN self-energy by each phonon mode allow us to verify which mode contributes the most to the ZPR. In addition, introducing the phonon frequencies at Γ, except the acoustic modes, we can compare the coupling strength for each mode as it is done in the generalized Fröhlich model,

$$\mathrm{ZPR}_{\mathbf{k}n} = \sum_j \alpha_j \omega_{j0} \tag{S.4}$$

where $\alpha_j = \mathrm{ZPR}_{j\mathbf{k}n}/\omega_{j0}$.

The DW self-energy is determined using the acoustic sum rule within the rigid-ion approximation[1], and its formulation is detailed in Ref. 9.

### S. A. Supplementary tables

In table S.2, the frequencies average $\langle\omega_{j0}\rangle_{\mathrm{ZPR}}$ is calculated using the ZPR values as weights, $\sum_j \omega_{j0} \times \mathrm{ZPR}_j/\mathrm{ZPR}$, where the sum is over the phonon modes and the ZPR with or without index discerns between per phonon mode and the total, respectively. All other averages in the table are over $\hat{\mathbf{q}}$.

| Material | $\varepsilon^*_{sFr}$ | $\omega_{LO}$ | $\langle m_* \rangle$ | $\alpha$ | ZPR |
|---|---|---|---|---|---|
| $RbN_3$ | 4.713 | 265 | 1.175 | 1.646 | -437 |
| | | | (1.974) | (2.135) | (547) |
| $KN_3$ | 4.705 | 267 | 1.107 | 1.680 | -448 |
| | | | (1.225) | (2.049) | (546) |
| $NaN_3$ | 4.484 | 272 | 1.201 | 1.727 | -471 |
| | | | (2.608) | (2.545) | (693) |
| $LiN_3$ | 4.245 | 276 | 1.858 | 2.253 | -623 |
| | | | (2.938) | (2.834) | (783) |
| $Cs_2NaScF_6$ | 3.449 | 63 | 8.827 | 12.659 | -798 |
| | | | (6.081) | (10.507) | (662) |
| $CsNO_2$ | 4.039 | 163 | 3.467 | 4.208 | -687 |
| | | | (5.244) | (5.176) | (845) |
| $Li_2CaHfF_8$ | 3.256 | 73 | 22.269 | 19.829 | -1441 |
| | | | (7.398) | (11.432) | (831) |
| $K_2TiF_6$ | 3.046 | 82 | 10.436 | 13.633 | -1123 |
| | | | (8.199) | (12.083) | (995) |

TABLE S.1: Parameters for the standard Fröhlich model. The effective masses $m^*$ at the CBM(VBM) were calculated using Eq. (23). $\omega_{LO}$ is the highest phonon frequency in meV, $\alpha$ is the electron-phonon coupling constant for the CBM(VBM), and the ZPR was determined at the CBM(VBM) in meV.

| Material | $\langle \varepsilon^*_j(\hat{\mathbf{q}}) \rangle$ | $\langle \omega_{j0} \rangle_{\mathrm{ZPR}}$ | $\langle \alpha_j(\hat{\mathbf{q}}) \rangle$ | ZPR |
|---|---|---|---|---|
| $RbN_3$ | 3.885 | 71 | 6.821 | -172 |
| | | | (8.811) | (222) |
| $KN_3$ | 3.891 | 73 | 6.333 | -192 |
| | | | (7.740) | (234) |
| $NaN_3$ | 3.433 | 59 | 6.746 | -241 |
| | | | (8.917) | (325) |
| $LiN_3$ | 3.061 | 66 | 8.166 | -422 |
| | | | (8.000) | (436) |
| $Cs_2NaScF_6$ | 2.817 | 48 | 20.452 | -787 |
| | | | (16.293) | (627) |
| $CsNO_2$ | 1.169 | 23 | 78.737 | -742 |
| | | | (94.277) | (913) |
| $Li_2CaHfF_8$ | 2.608 | 66 | 28.132 | -1580 |
| | | | (17.287) | (964) |
| $K_2TiF_6$ | 2.483 | 57 | 25.871 | -986 |
| | | | (23.743) | (908) |

TABLE S.2: Parameters for the generalized Fröhlich model. The dielectric constant and $\alpha$ are averaged over $\mathbf{q}$ and phonon mode, $j$. The phonon frequencies ( in meV) are averaged over $j$ using the ZPR per mode as probabilistic weight. The ZPR is also given in meV. The calculations were done for the states CBM and (VBM).

| Phonon mode | $\omega_\Gamma$ (meV) | $ZPR_i$ (meV) | (%) to $ZPR_i$ | $\alpha_i$ |
|---|---|---|---|---|
| 15 | 28 | 62.0 | 26.14 | 2.57 |
| 17 | 80 | 33.5 | 14.12 | 0.42 |
| 19 | 81 | 11.4 | 4.79 | 0.14 |
| 20 | 81 | 18.3 | 7.70 | 0.22 |
| 21 | 168 | 34.0 | 14.33 | 0.20 |
| 22 | 169 | 38.0 | 16.05 | 0.23 |
| 24 | 271 | 14.0 | 5.89 | 0.05 |
| 15 | 20 | 145.2 | 75.97 | 5.84 |
| 24 | 260 | 36.8 | 19.27 | 0.14 |

TABLE S.3: Contributions of different phonon modes (24 in total) to the full $ZPR_c$ of $KN_3$. Top 7 rows are the non-adiabatic AHC results (all types of modes) and the bottom 2 rows are the generalized Fröhlich (only LO modes). Only phonon modes that contribute more than 4% are shown, summing to a total of 89% for AHC and 95% for the generalized Fröhlich model.

| Phonon mode | $\omega_\Gamma$ (meV) | ZPR$_i$ (meV) | (%) to ZPR$_i$ | $\alpha_i$ |
|---|---|---|---|---|
| 18 | 26 | 98.5 | 10.07 | 5.26 |
| 24 | 33 | 58.8 | 6.02 | 1.98 |
| 29 | 59 | 439.7 | 44.97 | 9.20 |
| 30 | 63 | 278.4 | 28.47 | 5.07 |
| 12 | 15 | 50.5 | 6.42 | 3.48 |
| 18 | 26 | 116.4 | 14.78 | 4.48 |
| 24 | 33 | 179.6 | 22.81 | 5.50 |
| 30 | 63 | 440.8 | 55.99 | 6.99 |

TABLE S.4: Contributions of different phonon modes (30 in total) to the full ZPR$_c$ of $Cs_2NaScF_6$. Top 4 rows are the non-adiabatic AHC results (all types of modes) and the bottom 4 rows are the generalized Fröhlich data (only LO modes). Only phonon modes contributing more than 4% are shown (accounting for 90% of the total).

| | Electron | | Hole | |
|---|---|---|---|---|
| | $\alpha < 6$ | $\alpha \geq 6$ | $\alpha < 6$ | $\alpha \geq 6$ |
| $a_P \geq 10$ | 94.91 % | 0.08 % | 64.89 % | 0.56 % |
| $a_P < 10$ | 3.50 % | 1.51 % | 19.43 % | 15.13 % |

TABLE S.5: Distribution of electron and hole polarons in the four quadrants based on their respective radii and coupling strength.

| Material | Latt. | $< m^* >$ | $\omega_{LO}$(meV) | $\epsilon^\infty$ | $\epsilon^0$ | ZPR$_v^{gFr}$(meV) |
|---|---|---|---|---|---|---|
| AlAs | zb | 0.223 | 47.3 | 9.49 | 11.51 | 11.50 |
| AlP | zb | 0.342 | 59.9 | 8.12 | 10.32 | 20.56 |
| AlSb | zb | 0.163 | 39.8 | 12.02 | 13.35 | 4.00 |
| BAs | zb | 0.230 | 84.4 | 9.81 | 9.89 | 0.53 |
| BN | zb | 0.525 | 161.0 | 4.52 | 6.69 | 94.47 |
| CdS | zb | 0.288 | 34.4 | 6.21 | 10.24 | 38.73 |
| CdSe | zb | 0.138 | 23.6 | 7.83 | 11.78 | 19.69 |
| CdTe | zb | 0.133 | 19.1 | 8.89 | 12.37 | 11.91 |
| GaAs | zb | 0.026 | 33.5 | 15.31 | 17.55 | 3.27 |
| GaN | zb | 0.333 | 86.0 | 6.13 | 16.30 | 72.26 |
| GaP | zb | 0.209 | 48.6 | 10.50 | 11.00 | 8.46 |
| SiC | zb | 0.488 | 117.0 | 6.97 | 10.30 | 58.28 |
| ZnS | zb | 0.362 | 40.6 | 5.97 | 9.40 | 40.06 |
| ZnSe | zb | 0.217 | 29.3 | 7.35 | 10.73 | 21.69 |
| ZnTe | zb | 0.175 | 24.1 | 9.05 | 11.99 | 11.06 |
| CaO | rs | 0.855 | 66.8 | 3.77 | 16.76 | 223.20 |
| $Li_2O$ | rs | 1.369 | 86.3 | 2.9 | 7.8 | 364.59 |
| MgO | rs | 0.855 | 84.5 | 3.23 | 11.14 | 326.99 |
| SrO | rs | 0.853 | 55.4 | 3.77 | 20.91 | 228.95 |

TABLE S.6: Calculated valence band ZPR for selected cubic materials as in Miglio et al.[10] in the generalized Fröhlich formalism ($ZPR_v^{gFr}$) based on first principles GGA-PBE parameters. For such simple materials, the generalized Fröhlich model and the standard Fröhlich model with the hypotheses laid in Sec. II are equivalent. The materials considered contain triply degenerated valence bands coupled to one LO phonon branch. The lattice types abbreviations correspond to zinc-blende(zb), respectively rocksalt(rs) thus belonging to the cubic space group symmetry.

### S. B. Supplementary figures

The convergence of the electron-phonon interactions in terms of the $N \times N \times N$ **q**-grid mesh is obtained by extrapolation to a mesh of infinite number of **q**-points or, similarly, to $1/N \to 0$. In Fig. S.1, we extract the ZPR$_c$ of the four azides for $1/N \to 0$ with a linear fit of the three densest **q**-grid meshes, where N=8, 16, 32, and 64. The same procedure was used for $Cs_2NaScF_6$ in Fig. S.2 and for the other materials specified in Section IV.

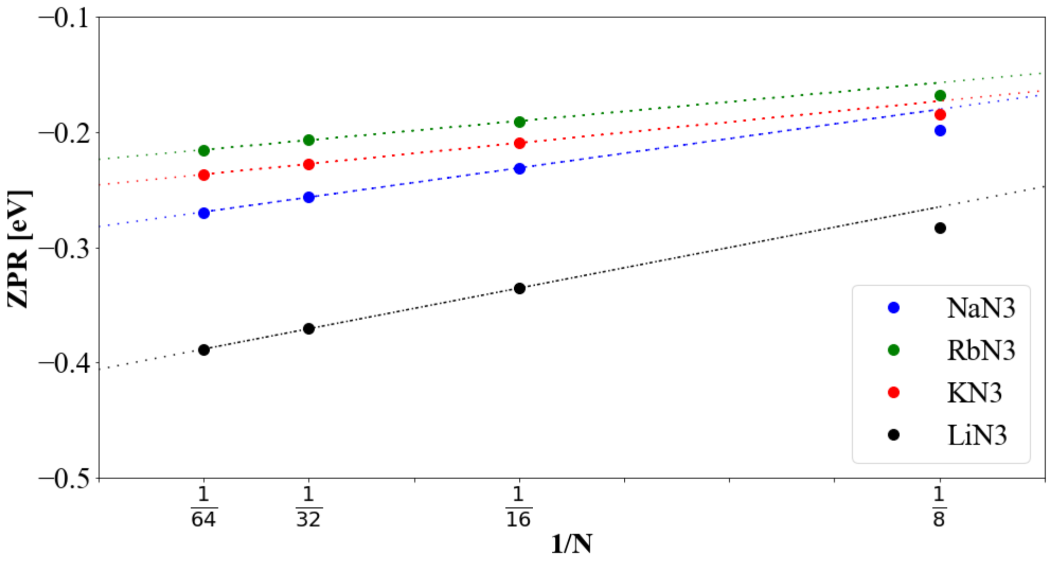


FIG. S.1: Convergence of the ZPR$_c$ of $LiN_3$, $NaN_3$, $KN_3$ and $RbN_3$, as a function of the phonon wavevector **q**-grid density N×N×N. The data is extrapolated linearly with respect to $1/N$ by fitting the values at $N = 16$, 32 and 64.

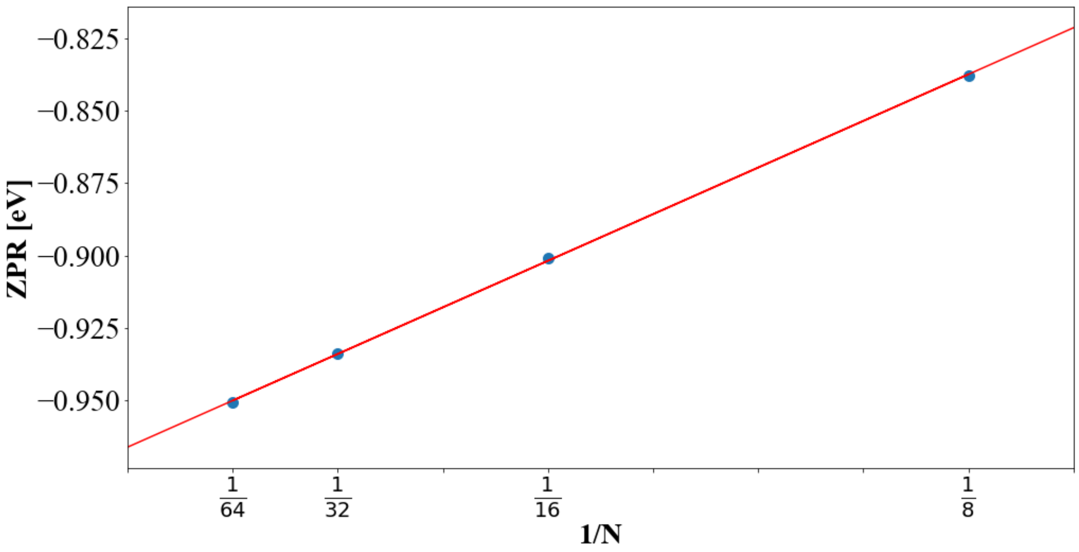


FIG. S.2: Convergence of the ZPR$_c$ of $Cs_2NaScF_6$ as a function of the phonon wavevector **q**-grid density N×N×N. The data is extrapolated linearly with respect to $1/N$, fitting the four visible grid densities.

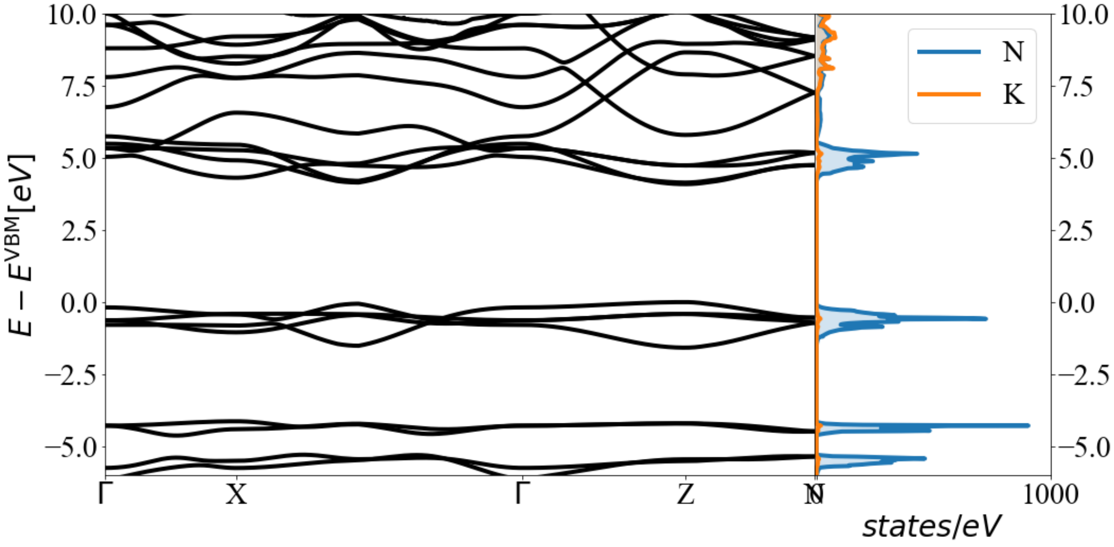


FIG. S.3: Electronic band structure of $KN_3$. The band masses are not extremely large, but the conduction and valence edges are made from purely Nitrogen orbitals, with localized molecular-like states, which lead to the very flat phonon bands, large frequencies, and very strong electron phonon coupling.

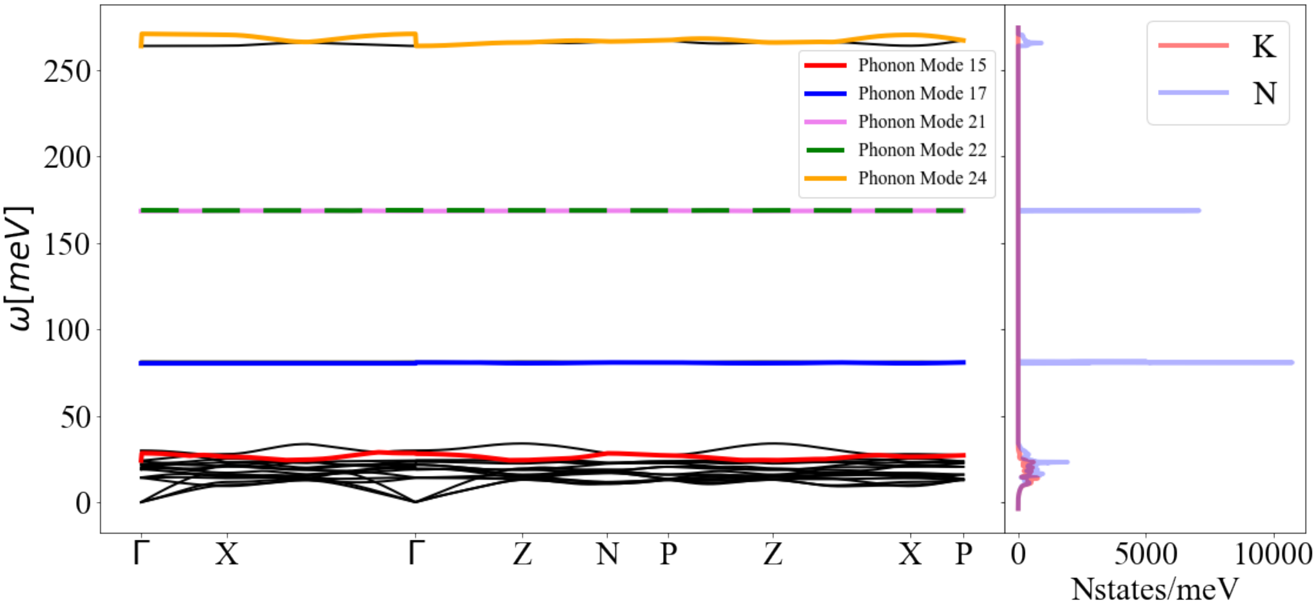


FIG. S.4: Phonon band structure of $KN_3$ (left) and the projected density of states (right). On the phonon band structure, the four phonon modes with the highest contribution to the $ZPR_c$ are shown with colored lines. The phonon modes 21 and 22 are almost degenerate.

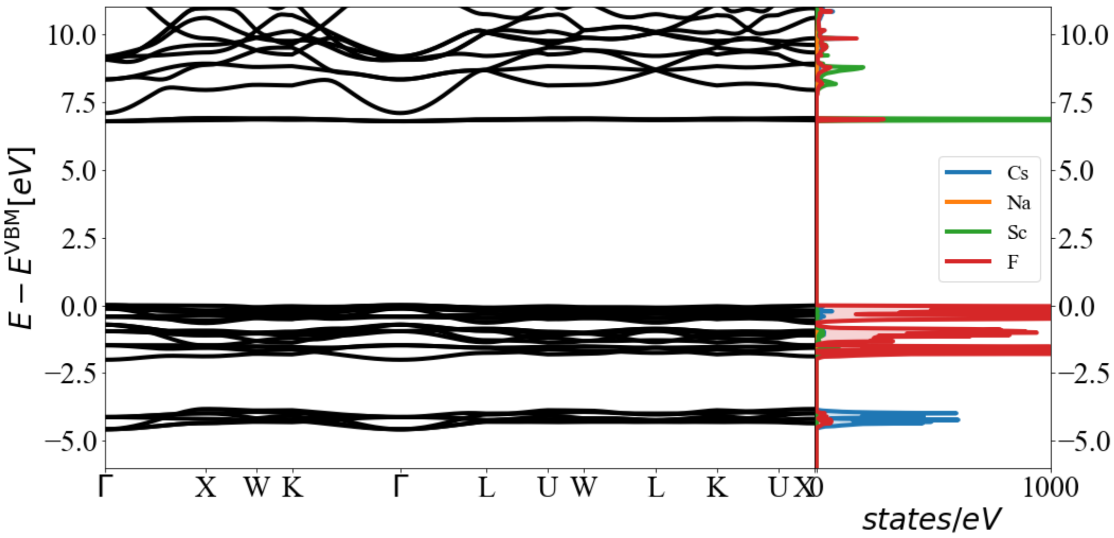


FIG. S.5: Electronic band structure of $Cs_2NaScF_6$. The bottom conduction band is almost flat, being a pure Sc d band emptied by the very aggressive electrophilic F atoms, and split off from the rest of the conduction band as an ideal impurity level.

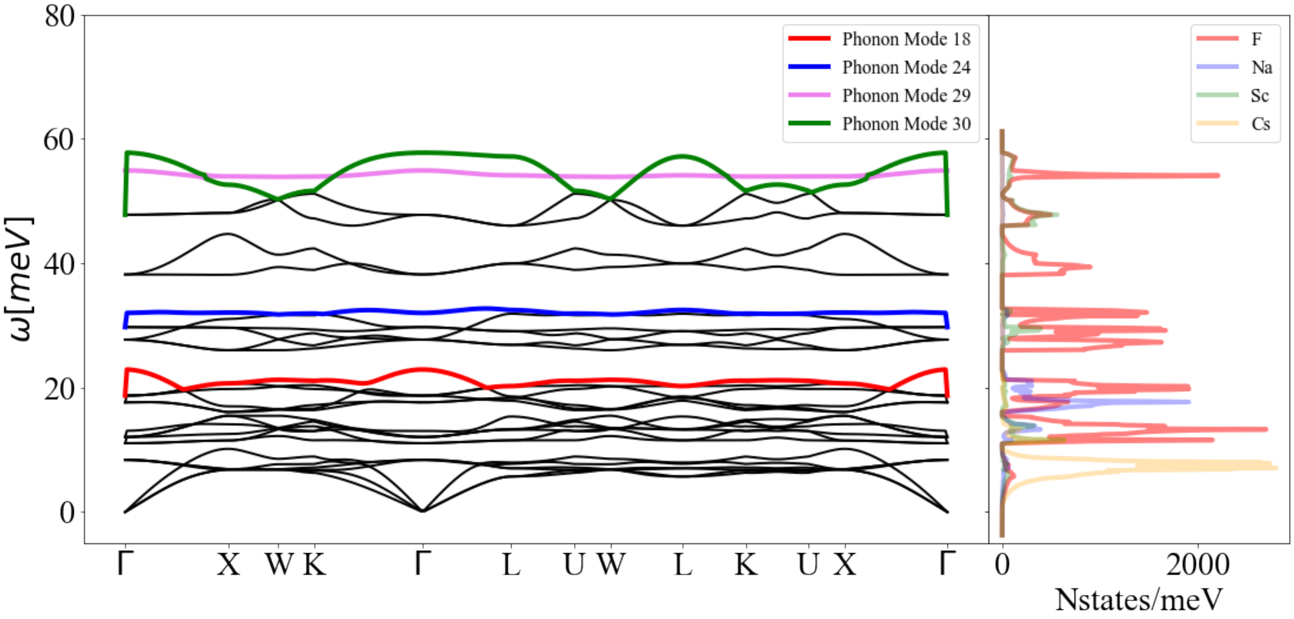


FIG. S.6: Phonon band structure of $Cs_2NaScF_6$ (left) and the projected density of states (right). On the phonon band structure, the four phonon modes with the highest contribution to the $ZPR_c$ are shown as colored lines. The pink horizontal line for mode 29 is identified by continuity of atomic character, and leads to a very narrow peak in the DOS.

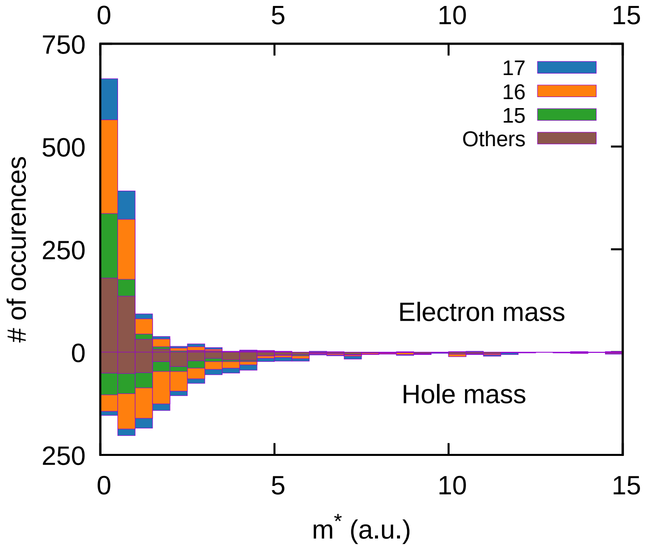


FIG. S.7: Hole and electron effective mass distribution. Stacked bars correspond to compounds containing elements from certain chemical groups.

### S. C. Full results from high-throughput calculations


[1] P. B. Allen and V. Heine. Theory of the temperature dependence of electronic band structures. *J. Phys. C*, 9:2305–2312, 1976.

[2] P. B. Allen and M. Cardona. Theory of the temperature dependence of the direct gap of germanium. *Phys. Rev. B*, 23:1495–1505, 1981.

[3] A. B. Migdal. Interaction between electrons and lattice vibrations in a normal metal. *Zh. Eksp. Teor. Fiz.*, 34:1438, 1958.

[4] E. Antoncik. On the theory of temperature shift of the absorption curve in non-polar crystals. *Czechoslovak Journal of Physics*, 5:449, 1955.

[5] H. Y. Fan. Temperature dependence of the energy gap in semiconductors. *Phys. Rev.*, 82:900–905, 1951.

[6] M. Royo and M. Stengel. First-Principles Theory of Spatial Dispersion: Dynamical Quadrupoles and Flexoelectricity . *Phys. Rev. X*, 9:021050, 2019.

[7] Guillaume Brunin, Henrique Pereira Coutada Miranda, Matteo Giantomassi, Miquel Royo, Massimiliano Stengel, Matthieu J. Verstraete, Xavier Gonze, Gian-Marco Rignanese, and Geoffroy Hautier. Electron-phonon beyond fröhlich: dynamical quadrupoles in polar and covalent solids. *Phys. Rev. Lett.*, 125:136601, 2020.

[8] Guillaume Brunin, Henrique Pereira Coutada Miranda, Matteo Giantomassi, Miquel Royo, Massimiliano Stengel, Matthieu J. Verstraete, Xavier Gonze, Gian-Marco Rignanese, and Geoffroy Hautier. Phonon-limited electron mobility in si, gaas and gap with exact treatment of dynamical quadrupoles. *Phys. Rev. B*, 102:094308, 2020.

[9] S. Poncé, Y. Gillet, J. Laflamme Janssen, A. Marini, M. Verstraete, and X. Gonze. Temperature dependence of the electronic structure of semiconductors and insulators. *J. Chem. Phys.*, 143(10):102813, 2015.

[10] Anna Miglio, Véronique Brousseau-Couture, Emile Godbout, Gabriel Antonius, Yang-Hao Chan, Steven G. Louie, Michel Côté, Matteo Giantomassi, and Xavier Gonze. Predominance of non-adiabatic effects in zero-point renormalization of the electronic band gap. *npj Computational Materials*, 6(1):167, 2020.

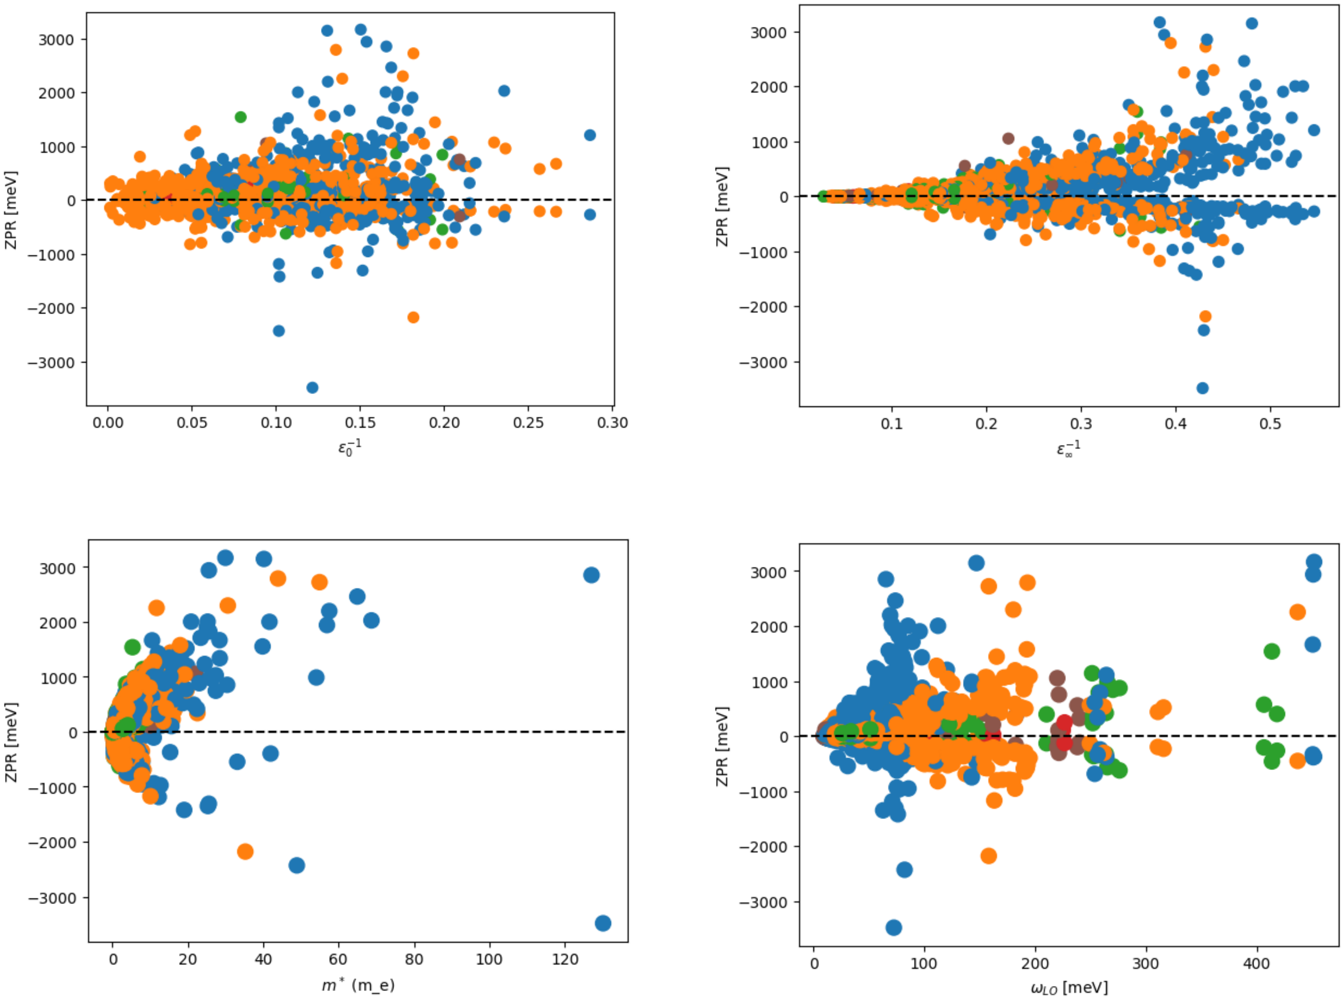


FIG. S.8: Values of conduction (negative) and valence (positive) ZPR$^{\mathrm{sFR}}$ for all materials versus $\epsilon_0^{-1}$ (top-left), $\epsilon_\infty^{-1}$ (top-right), $m^*$ (bottom-left), and $\omega_{\mathrm{LO}}$ (bottom-right).

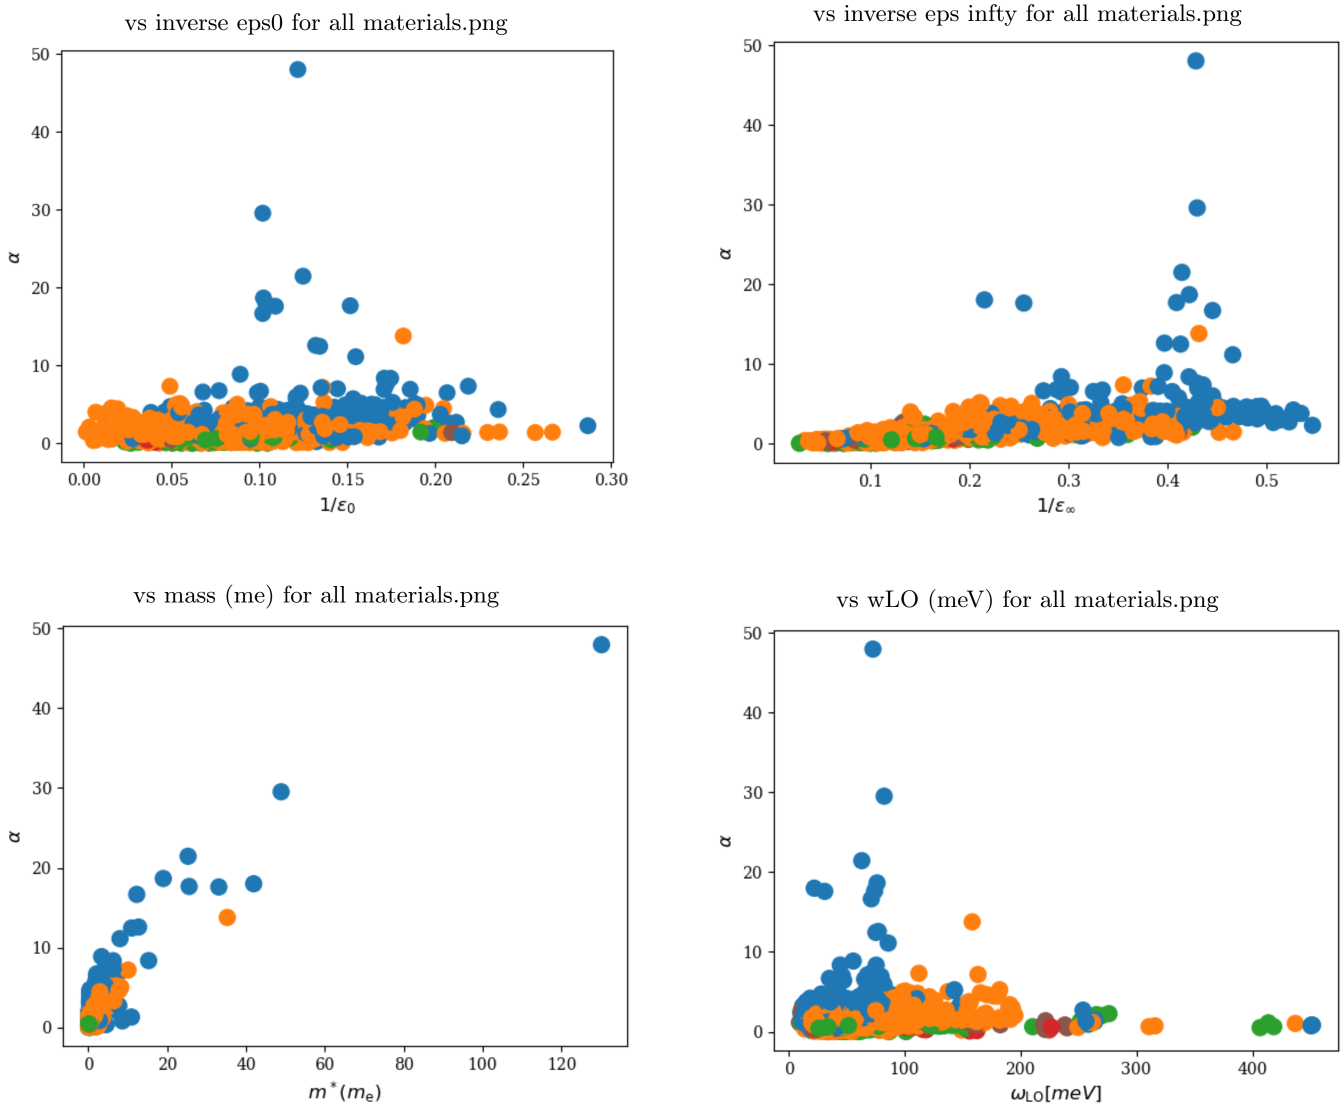


FIG. S.9: Values of conduction and valence $\alpha^{\mathrm{sFR}}$ for all materials versus $\epsilon_0^{-1}$ (top-left), $\epsilon_\infty^{-1}$ (top-right), $m^*$ (bottom-left), and $\omega_{\mathrm{LO}}$ (bottom-right).
